# Supplementary material for: Pareto-Conditioned Diffusion Models for Offline Multi-Objective Optimization
Source: arXiv:2602.00737 source file (2026-02-13)
Supplement: Supplementary file 1 [file d_best_cond.tex]

\begin{tabular}{lcccc}
\toprule
Method & C10/MOP2 & MO-Hopper-v2 & RE34 & ZDT2 & Regex\\
\midrule
D(best) + N/A & 10.44$\pm$0.02 & 6.19$\pm$0.54 & 9.32$\pm$0.01 & 7.53$\pm$0.41 & NA\\
D(best) + Reweight & 10.57$\pm$0.04 & 6.11$\pm$0.33 & 9.85$\pm$0.39 & 6.57$\pm$0.24 & NA\\
\bottomrule
\end{tabular}
