# Supplementary material for: Pareto-Conditioned Diffusion Models for Offline Multi-Objective Optimization
Source: arXiv:2602.00737 source file (2026-02-13)
Supplement: Supplementary file 2 [file m_objective_cost.tex]

\begin{tabular}{lcccc}
\toprule
& \multicolumn{4}{c}{No. objectives} \\
\cmidrule(lr){2-5}
Task & 3 & 4 & 5 & 6 \\
\midrule
DTLZ1 & 15.03 $\pm$ 0.04 & 17.51 $\pm$ 0.04 & 18.48 $\pm$ 0.21 & 29.07 $\pm$ 0.44 \\
DTLZ7 & 17.08 $\pm$ 0.02 & 16.72 $\pm$ 0.02 & 18.24 $\pm$ 0.23 & 28.12 $\pm$ 0.30 \\
\bottomrule
\end{tabular}
