# Supplementary material for: Pareto-Conditioned Diffusion Models for Offline Multi-Objective Optimization
Source: arXiv:2602.00737 source file (2026-02-13)
Supplement: Supplementary file 4 [file training_details.tex]

\begin{tabular}{c|ccccc}
    \toprule
    Parameter & Synthetic & MORL & RE & Scientific & MONAS\\
    \midrule
    \multicolumn{6}{c}{Model parameters}\\
    \midrule
    \# of training steps & 1000 & 4000 & 4000 & 1000 & 1000 \\
    Learning rate & $3e-4$ & $3e-4$ & $3e-4$ & $3e-4$ & $3e-4$ \\
    \# of layers & 4 & 4 & 4 & 4  & 4 \\
    \# Neurons / layer & 512 & 512 & 512 & 512 & 512\\
    \midrule
    \multicolumn{6}{c}{Sampling parameters}\\
    \midrule
    \# of sampling steps & 1024 & 1024 & 1024 & 1024  & 1024 \\
    \# Neurons / layer & 512 & 512 & 512 & 512 & 512\\
    \midrule
    \midrule
    \multicolumn{6}{c}{Reweighting parameters}\\
    \midrule
    \# Bins & 30 & 30 & 30 & 30  & 30 \\
    K & 10 & 10 & 10 & 10 & 10 \\
    $\tau$ & 0.05 & 0.05 & 0.05 & 0.05 & 0.05 \\
    \bottomrule
\end{tabular}
